# Supplementary material for: Advancing Ad Auction Realism: Practical Insights & Modeling Implications
Source: arXiv:2307.11732 source file (2024-04-09)
Supplement: Supplementary file 1 [file appendix.tex]

\section{Appendix}
\label{sec:appendix}

\subsection{Asymmetric value distribution}
\label{asym_value}

The following tables provide numerical values for the Figures~1-3 in \S\ref{sfrp_vs_rp}. 

%%%%%%%%%%%%%%%%%%%%%%%%
\begin{table}[ht]
\raggedright
\captionsetup{justification=raggedright,singlelinecheck=false}
\caption{Beta(4,1) right-skewed value distribution}
\label{tab:my-table}
\vspace{0.1in}
\begin{tabular}{|c|c|c|c|c|}
\hline
Reserve & Exp Rev SF & Stdev & Exp Rev RP & Stdev \\
\hline
0       & 1.1507     & 0.0002  &            &       \\
0.2     & 1.1692     & 0.0002  & 1.1641     & 0.0002 \\
0.4     & 1.1556     & 0.0002  & 1.1911     & 0.0002 \\
0.6     & 1.1787     & 0.0004  & 1.1502     & 0.0003 \\
0.8     & 1.1533     & 0.0368  & 1.1604     & 0.0001 \\
1       & 0.9139     & 0.0056  & 1.0005     & 0.0002 \\
1.2     & 1.0117     & 0.0043  &            &       \\
1.4     & 1.0711     & 0.0577  &            &       \\
1.6     & 1.1688     & 0.061   &            &       \\
1.8     & 1.0203     & 0.1095  & 1.3974     & 0.0008 \\
2       & 1.1573     & 0.06    & 0.0479     & 0.0009 \\
2.2     & 1.1384     & 0.0684  & 0          & 0     \\
\hline
\end{tabular}
\end{table}

%%%%%%%%%%%%%%%%%%%%%%%%
\begin{table}[ht]
\raggedright
\captionsetup{justification=raggedright,singlelinecheck=false}
\caption{Beta(3,1) right-skewed value distribution}
\vspace{0.1in}
\begin{tabular}{|c|c|c|c|c|}
\hline
Reserve & Exp Rev SF & Stdev & Exp Rev RP & Stdev \\
\hline
0       & 1.141      & 0.0003 &           &       \\
0.2     & 1.1307     & 0.0002 & 1.149     & 0.0001 \\
0.4     & 1.138      & 0.0003 & 1.1492    & 0.0003 \\
0.6     & 1.1358     & 0.0057 & 1.1361    & 0.0002 \\
0.8     & 1.0364     & 0.0016 & 1.1145    & 0.0002 \\
1       & 0.893      & 0.0076 & 1.0274    & 0.0003 \\
1.2     & 0.9997     & 0.0015 &           &       \\
1.4     & 1.0605     & 0.0561 &           &       \\
1.6     & 1.0946     & 0.0827 &           &       \\
1.8     & 1.1252     & 0.0698 & 1.3706    & 0.0006 \\
2       & 1.1146     & 0.0949 & 0.0469    & 0.0009 \\
2.2     & 1.0749     & 0.0873 & 0         & 0     \\
\hline
\end{tabular}
\end{table}

%%%%%%%%%%%%%%%%%%%%%%%%
\begin{table}[ht]
\raggedright
\captionsetup{justification=raggedright,singlelinecheck=false}
\caption{Beta(3,2) right-skewed value distribution}
\vspace{0.1in}
\begin{tabular}{|c|c|c|c|c|}
\hline
Reserve & Exp Rev SF & Stdev & Exp Rev RP & Stdev \\
\hline
0       & 0.9505     & 0.0002 &           &       \\
0.2     & 0.9637     & 0.0002 & 0.956     & 0.0002 \\
0.4     & 0.9565     & 0.0054 & 0.9549    & 0.0005 \\
0.6     & 0.9005     & 0.0011 & 0.9338    & 0.0001 \\
0.8     & 0.6692     & 0.0068 & 0.8938    & 0.0001 \\
1       & 0.7748     & 0.0123 & 0.9107    & 0.0002 \\
1.2     & 0.7706     & 0.0652 &           &       \\
1.4     & 0.8061     & 0.1406 &           &       \\
1.6     & 0.8759     & 0.1231 &           &       \\
1.8     & 0.8445     & 0.1048 & 1.3787    & 0.0006 \\
2       & 0.8512     & 0.1118 & 0.0471    & 0.0008 \\
2.2     & 0.8001     & 0.1129 & 0         & 0     \\
\hline
\end{tabular}
\end{table}

%%%%%%%%%%%%%%%%%%%%%%%%

\begin{table}[ht]
\raggedright
\captionsetup{justification=raggedright,singlelinecheck=false}
\caption{Beta(2,2) symmetric value distribution}
\vspace{0.1in}
\begin{tabular}{|c|c|c|c|c|}
\hline
Reserve & Exp Rev SF & Stdev & Exp Rev RP & Stdev \\
\hline
0       & 0.8985     & 0.0002 &           &       \\
0.2     & 0.9108     & 0.0002 & 0.913     & 0.0002 \\
0.4     & 0.854      & 0.0172 & 0.9109    & 0.0002 \\
0.6     & 0.8007     & 0.1639 & 0.8779    & 0.0003 \\
0.8     & 0.6502     & 0.0117 & 0.9014    & 0.0003 \\
1       & 0.7333     & 0.0109 & 0.9822    & 0.0001 \\
1.2     & 0.8286     & 0.0795 &           &       \\
1.4     & 0.7826     & 0.0991 &           &       \\
1.6     & 0.8817     & 0.0388 &           &       \\
1.8     & 0.8149     & 0.1313 & 1.3694    & 0.0003 \\
2       & 0.8509     & 0.1181 & 0.0478    & 0.002 \\
2.2     & 0.8588     & 0.0706 & 0         & 0     \\
\hline
\end{tabular}
\end{table}

%%%%%%%%%%%%%%%%%%%%%%%%

\begin{table}[ht]
\raggedright
\captionsetup{justification=raggedright,singlelinecheck=false}
\caption{Beta(3,3) symmetric value distribution}
\vspace{0.1in}
\begin{tabular}{|c|c|c|c|c|}
\hline
Reserve & Exp Rev SF & Stdev & Exp Rev RP & Stdev \\
\hline
0       & 0.898      & 0.0001 &           &       \\
0.2     & 0.8905     & 0.0002 & 0.9035    & 0.0001 \\
0.4     & 0.8698     & 0.0148 & 0.8919    & 0.0001 \\
0.6     & 0.865      & 0.0029 & 0.8629    & 0.0004 \\
0.8     & 0.653      & 0.0127 & 0.8973    & 0.0001 \\
1       & 0.7478     & 0.035  & 0.9897    & 0.001  \\
1.2     & 0.8748     & 0.0818 &           &       \\
1.4     & 0.8866     & 0.0618 &           &       \\
1.6     & 0.7939     & 0.0958 &           &       \\
1.8     & 0.8905     & 0.0929 & 1.3907    & 0.0012 \\
2       & 0.7667     & 0.0509 & 0.0472    & 0.0012 \\
2.2     & 0.8274     & 0.0664 & 0         & 0     \\
\hline
\end{tabular}
\end{table}

%%%%%%%%%%%%%%%%%%%%%%%%
\begin{table}[ht]
\raggedright
\captionsetup{justification=raggedright,singlelinecheck=false}
\caption{Beta(4,4) symmetric value distribution}
\vspace{0.1in}
\begin{tabular}{|c|c|c|c|c|}
\hline
Reserve & Exp Rev SF & Stdev & Exp Rev RP & Stdev \\
\hline
0       & 0.8891     & 0.0002 &           &       \\
0.2     & 0.8768     & 0.0002 & 0.878     & 0.0004 \\
0.4     & 0.893      & 0.0059 & 0.8744    & 0.0003 \\
0.6     & 0.8831     & 0.0018 & 0.8489    & 0.0003 \\
0.8     & 0.6421     & 0.0272 & 0.8888    & 0.0002 \\
1       & 0.9006     & 0.1171 & 0.9762    & 0.0005 \\
1.2     & 0.81       & 0.0718 &           &       \\
1.4     & 0.8878     & 0.0613 &           &       \\
1.6     & 0.8725     & 0.0822 &           &       \\
1.8     & 0.7797     & 0.0982 & 1.3628    & 0.0013 \\
2       & 0.8501     & 0.0904 & 0.0479    & 0.0021 \\
2.2     & 0.7814     & 0.1516 & 0         & 0     \\
\hline
\end{tabular}
\end{table}

%%%%%%%%%%%%%%%%%%%%%%%%

\begin{table}[ht]
\raggedright
\captionsetup{justification=raggedright,singlelinecheck=false}
\caption{Beta(2,3) left-skewed value distribution}
\vspace{0.1in}
\begin{tabular}{|c|c|c|c|c|}
\hline
Reserve & Exp Rev SF & Stdev & Exp Rev RP & Stdev \\
\hline
0       & 0.8018     & 0.0002 &           &       \\
0.2     & 0.8162     & 0.0001 & 0.8099    & 0.0002 \\
0.4     & 0.7769     & 0.0001 & 0.8203    & 0.0001 \\
0.6     & 0.4967     & 0.0112 & 0.8278    & 0.0002 \\
0.8     & 0.5929     & 0.0038 & 0.8992    & 0.0002 \\
1       & 0.6374     & 0.0495 & 0.986     & 0.0001 \\
1.2     & 0.7363     & 0.0992 &           &       \\
1.4     & 0.7131     & 0.1714 &           &       \\
1.6     & 0.7178     & 0.1641 &           &       \\
1.8     & 0.7097     & 0.1557 & 1.3839    & 0.0001 \\
2       & 0.7257     & 0.1025 & 0.0459    & 0.0011 \\
2.2     & 0.7891     & 0.0997 & 0         & 0     \\
\hline
\end{tabular}
\end{table}

%%%%%%%%%%%%%%%%%%%%%%%%

\begin{table}[ht]
\raggedright
\captionsetup{justification=raggedright,singlelinecheck=false}
\caption{Beta(1,3) left-skewed value distribution}
\vspace{0.1in}
\begin{tabular}{|c|c|c|c|c|}
\hline
Reserve & Exp Rev SF & Stdev & Exp Rev RP & Stdev \\
\hline
0       & 0.7431     & 0.0005 &           &       \\
0.2     & 0.7721     & 0.0001 & 0.7549    & 0.0001 \\
0.4     & 0.7519     & 0      & 0.7693    & 0.0002 \\
0.6     & 0.5609     & 0.0486 & 0.8022    & 0.0001 \\
0.8     & 0.6237     & 0.0945 & 0.8896    & 0.0001 \\
1       & 0.6656     & 0.0962 & 0.9638    & 0.0002 \\
1.2     & 0.6454     & 0.1395 &           &       \\
1.4     & 0.6493     & 0.1509 &           &       \\
1.6     & 0.6258     & 0.1446 &           &       \\
1.8     & 0.6707     & 0.1273 & 1.347     & 0.0006 \\
2       & 0.7232     & 0.1404 & 0.0486    & 0.0022 \\
2.2     & 0.7602     & 0.1315 & 0         & 0     \\
\hline
\end{tabular}
\end{table}

%%%%%%%%%%%%%%%%%%%%%%%%
\begin{table}[ht]
\raggedright
\captionsetup{justification=raggedright,singlelinecheck=false}
\caption{Beta(1,4) left-skewed value distribution}
\vspace{0.1in}
\begin{tabular}{|c|c|c|c|c|}
\hline
Reserve & Exp Rev SF & Stdev & Exp Rev RP & Stdev \\
\hline
0       & 0.7262     & 0.0002 &           &       \\
0.2     & 0.6854     & 0.0003 & 0.7072    & 0.0001 \\
0.4     & 0.7373     & 0.0001 & 0.7344    & 0.0001 \\
0.6     & 0.5427     & 0.0206 & 0.7915    & 0.0004 \\
0.8     & 0.5667     & 0.0061 & 0.8978    & 0.0001 \\
1       & 0.6686     & 0.058  & 0.9993    & 0       \\
1.2     & 0.7079     & 0.1102 &           &       \\
1.4     & 0.7375     & 0.0761 &           &       \\
1.6     & 0.7326     & 0.0394 &           &       \\
1.8     & 0.7472     & 0.1505 & 1.4022    & 0.0001 \\
2       & 0.611      & 0.1498 & 0.0481    & 0.0021 \\
2.2     & 0.7163     & 0.0724 & 0         & 0     \\
\hline
\end{tabular}
\end{table}
